# Supplementary material for: Study of B0 -> D*- pi+ pi- pi+ and B0 -> D*- K+ pi- pi+ decays
Source: arXiv:1303.6861 source file (2013-03-27)
Supplement: Supplementary file 2 [file supplementary.tex]

\section{Inclusion of supplementary material}
\label{sec:Supplementary}

In some cases it is desirable to approve material that is
supplementary to that which is included in the main body of the paper.
For example, sometimes a short letter paper is written, but additional
figures that cannot be contained within the page limit should be
approved to be available to be shown in talks. As a reminder, only
approved material can be shown in public. Another use case is to
provide data tables.  Any supplementary material should be made
available in the circulation to the collaboration in a clearly marked
appendix to the main document.  Before the paper is submitted this
appendix must be removed, and the supplementary material is added
separately to the CDS entry.

Journals published through or by the AIP, such as Phys. Rev. Lett. and
Phys. Rev. D, support the use of
\href{http://www.aip.org/pubservs/epaps.html}{EPAPS}.  Their
description of relevant supplementary material includes
\begin{quote} {\it multimedia (e.g., movie files, audio files,
    animated .gifs, 3D rendering files), color figures, data tables,
    and text (e.g., appendices) that are too lengthy or of too limited
    interest for inclusion in the printed journal}.
\end{quote}
LHCb publications in those journals can make of EPAPS as appropriate.
However, note that there are some categories of supplementary
material, such as additional plots, that are not appropriate for
EPAPS.

The appendix containing supplementary material should not normally be
referred to in the main body of the text as it will not appear in
the final version.  An exception is for material that will be
available in EPAPS, where the
\href{http://www.aip.org/epaps/how_epaps_works.html#deposit}{AIP
  recommendation} is
\begin{quote} {\it Files are made available to users via links from
    the journal. Authors should include a reference in the form ``See
    supplementary material at [URL will be inserted by AIP] for [give
    brief description of material].''}
\end{quote}
However, in this template, an example of the formatting for an appendix
of supplementary material is given in
Appendix~\ref{sec:Supplementary-App}.
